# Supplementary material for: Multiclass Transductive Online Learning
Source: arXiv:2411.01634 source file (2024-11-03)
Supplement: Supplementary file 3 [file RW_Example.tex]

% Amirreza

\section{Real World Example}

Yet another example motivating our paper comes from the quantum world. Consider a quantum experiment involving $N \in \mathbb{N}$ qubits, where a finite number $T \in \mathbb{N}$ of measurements are planned at arbitrary but fixed times before the experiment begins. This setup results in a sequence of $T$ pairs, each consisting of measurement features and its respective time. Moreover, given that there are $N$ qubits, each measurement can result in one of $2^N$ possible outcomes. As the experiment progresses, predictions of the outcome are made prior to each measurement, followed by observing the actual results. In this context, a reasonable goal is to minimize the number of prediction errors. How can we effectively formalize and address this problem with minimal assumptions? % It's noteworthy to mention that predicting an $n$ digit binary number is only meaningful when we have a measurement.
